# Supplementary material for: Learning Social Graph for Inactive User Recommendation
Source: arXiv:2405.05288 source file (2024-05-22)
Supplement: Supplementary file 1 [file appendix.tex]

\section{Mimic Learning}
\label{Mimic LearningMimic Learning}
In the proposed LSIR, we introduce Mimic Learning technique to make model learn how to establish new connections for inactive users. Specifically, we manipulate embeddings of active user $\bm{e_{u_{+}}}$ to mimic the distribution of inactive ones via the following three ways:

\textbf{Random Mask.} The essence of changing is to reduce message contained in $\bm{e}_{u_{+}}$. In this sense, it is a natural way to randomly mask a fraction of dimensions with zeros in $\bm{e}_{u_{+}}$. Formally, we first sample a random vector $\bar{\bm{m}}\in\{0, 1\}^{d}$, where $d$ is the dimension size of $\bm{e}_{u_{+}}$. Each dimension of $\bar{\bm{m}}$ independently is drawn from a Bernoulli distribution. Then, the changed embedding is computed by $\bm{e}_{u_{+}}^{RM}=\bm{e}_{u_{+}}\circ\bar{\bm{m}}$, where $\circ$ is the element-wise multiplication.

\textbf{Distribution Shift.} In this branch, we mainly focus on separately modeling embedding distributions of active users and inactive users, and then transform the former one to the latter. Specifically, in one training epoch, we get a set of active users $S_+$ and a set of inactive users $S_{-}$. Then, we change $\bm{e}_{u_{+}}$ as following:
\begin{equation}
\label{ds}
\bm{e}_{u_{+}}^{DS}=\phi(S_{-})\frac{\bm{e}_{u_{+}}-\mu(S_{+})}{\phi(S_{+})}+\mu(S_{-}),
\end{equation}
where $\mu(S)$ and $\phi(S)$ calculate the mean and standard deviation of user embeddings in set $S$.

\textbf{Inactive Mixture.} MixUp~\cite{mixup} is proposed to efficiently improve results in supervised learning by adding arbitrary two samples to create a new one. MixGCF~\cite{mixgcf} introduces this strategy into graph-based recommendation, who involves positive samples into negative ones to generate harder negatives. Inspired by them, we inject inactive information into active embeddings. Firstly, for each active user $u_{+}$, we randomly select $\eta$ inactive users in one batch, and combine them with $u_{+}$ with weight $\beta\in(0,1)$:
\begin{equation}
\label{im}
\bm{e}_{u_{+}}^{IM}=\beta\bm{e}_{u_{+}}+(1-\beta)\bm{e}_{u_{-}},
\end{equation}
where $\bm{e}_{u_{-}}$ is embedding of one selected inactive user.

\begin{wrapfigure}[9]{r}{0.6\textwidth}
\centering
    \vspace{-20pt}
    \subfigure[Flickr]
{
    \begin{minipage}[b]{.25\textwidth}
        \centering
        \includegraphics[width=\textwidth]{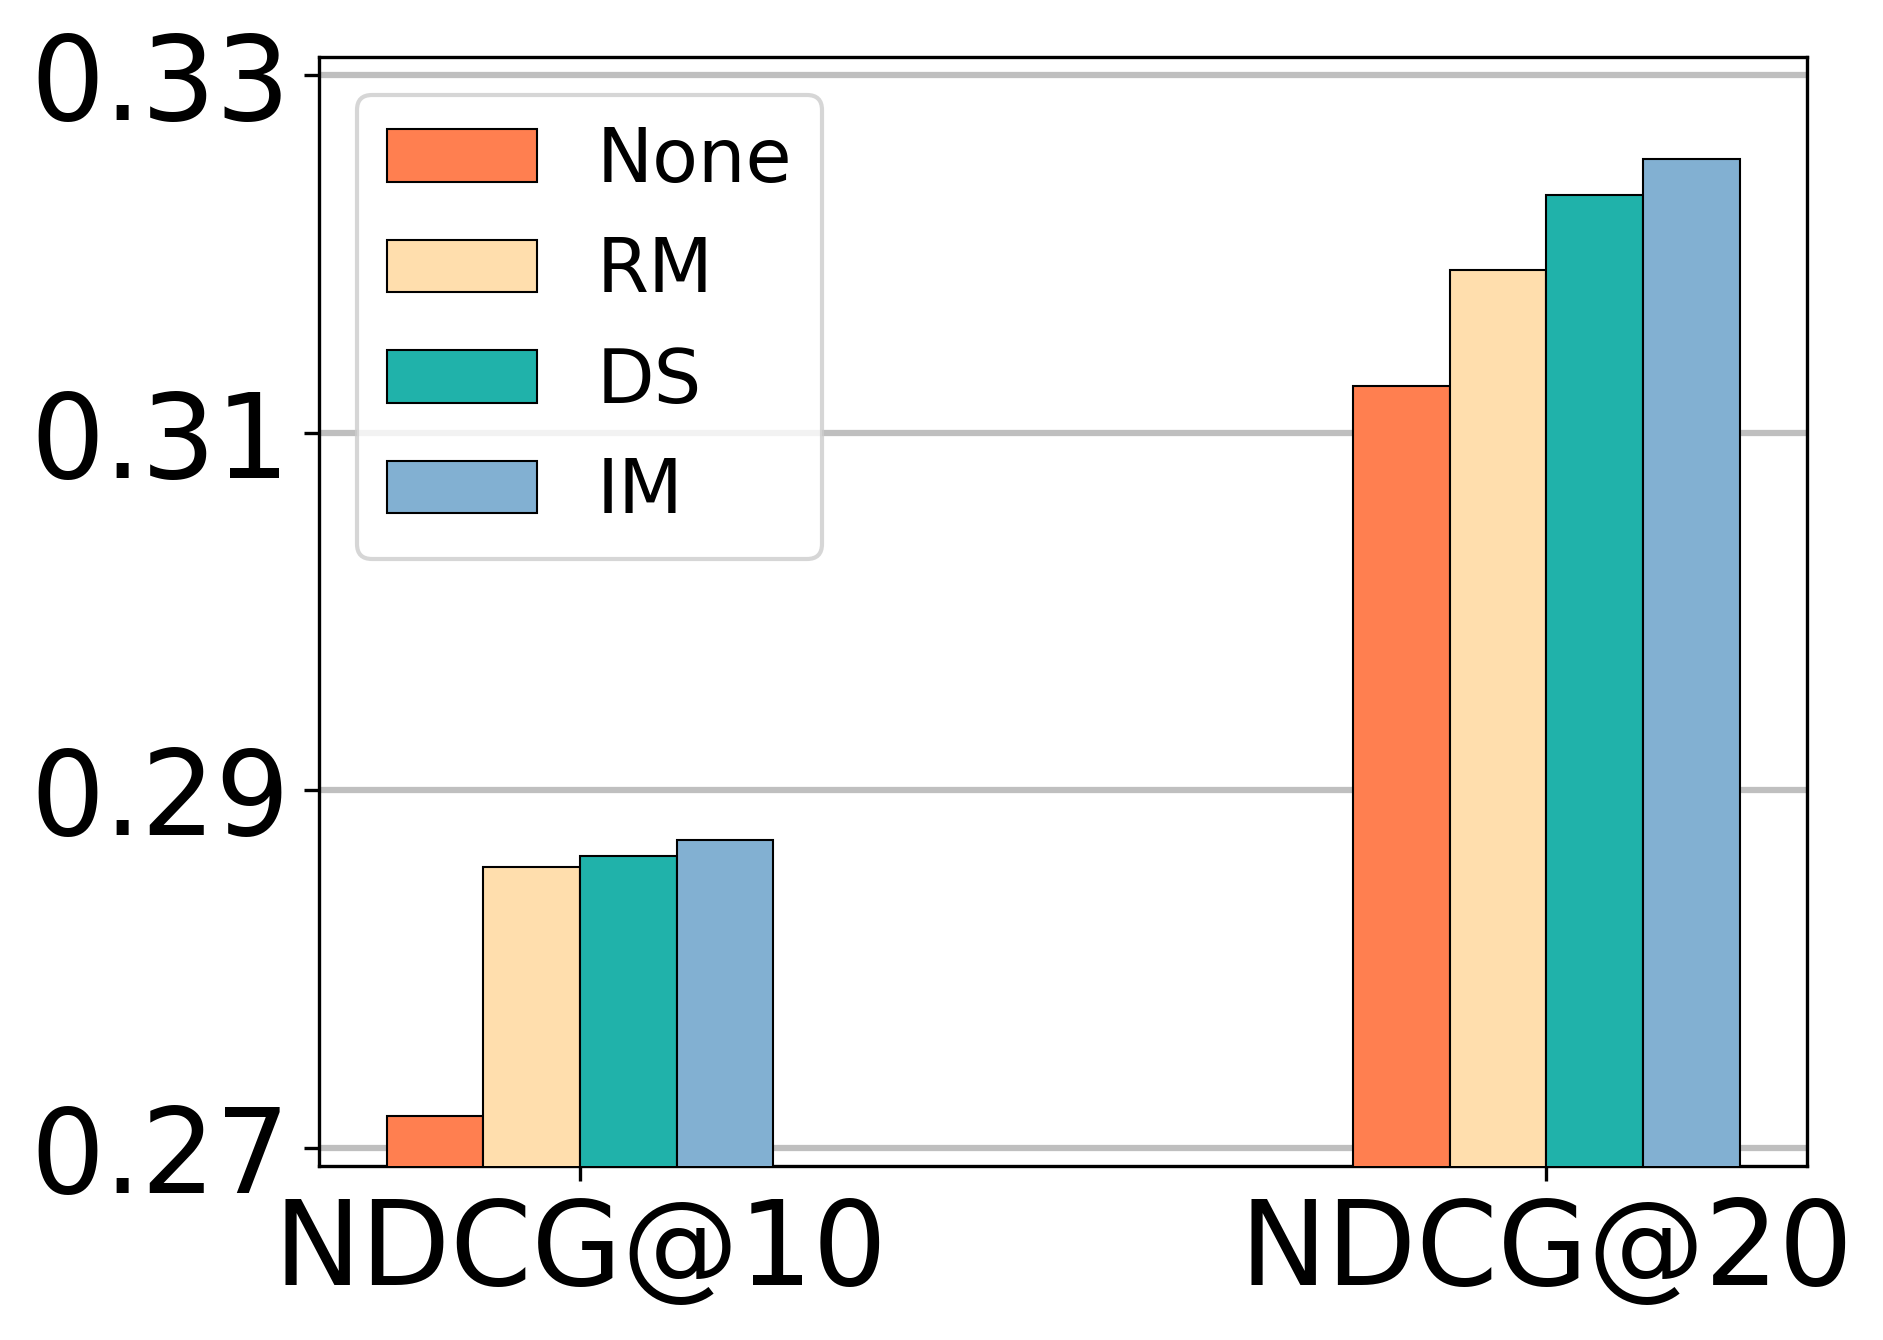}
    \end{minipage}
}
\subfigure[Yelp]
{
 	\begin{minipage}[b]{.25\textwidth}
        \centering
        \includegraphics[width=\textwidth]{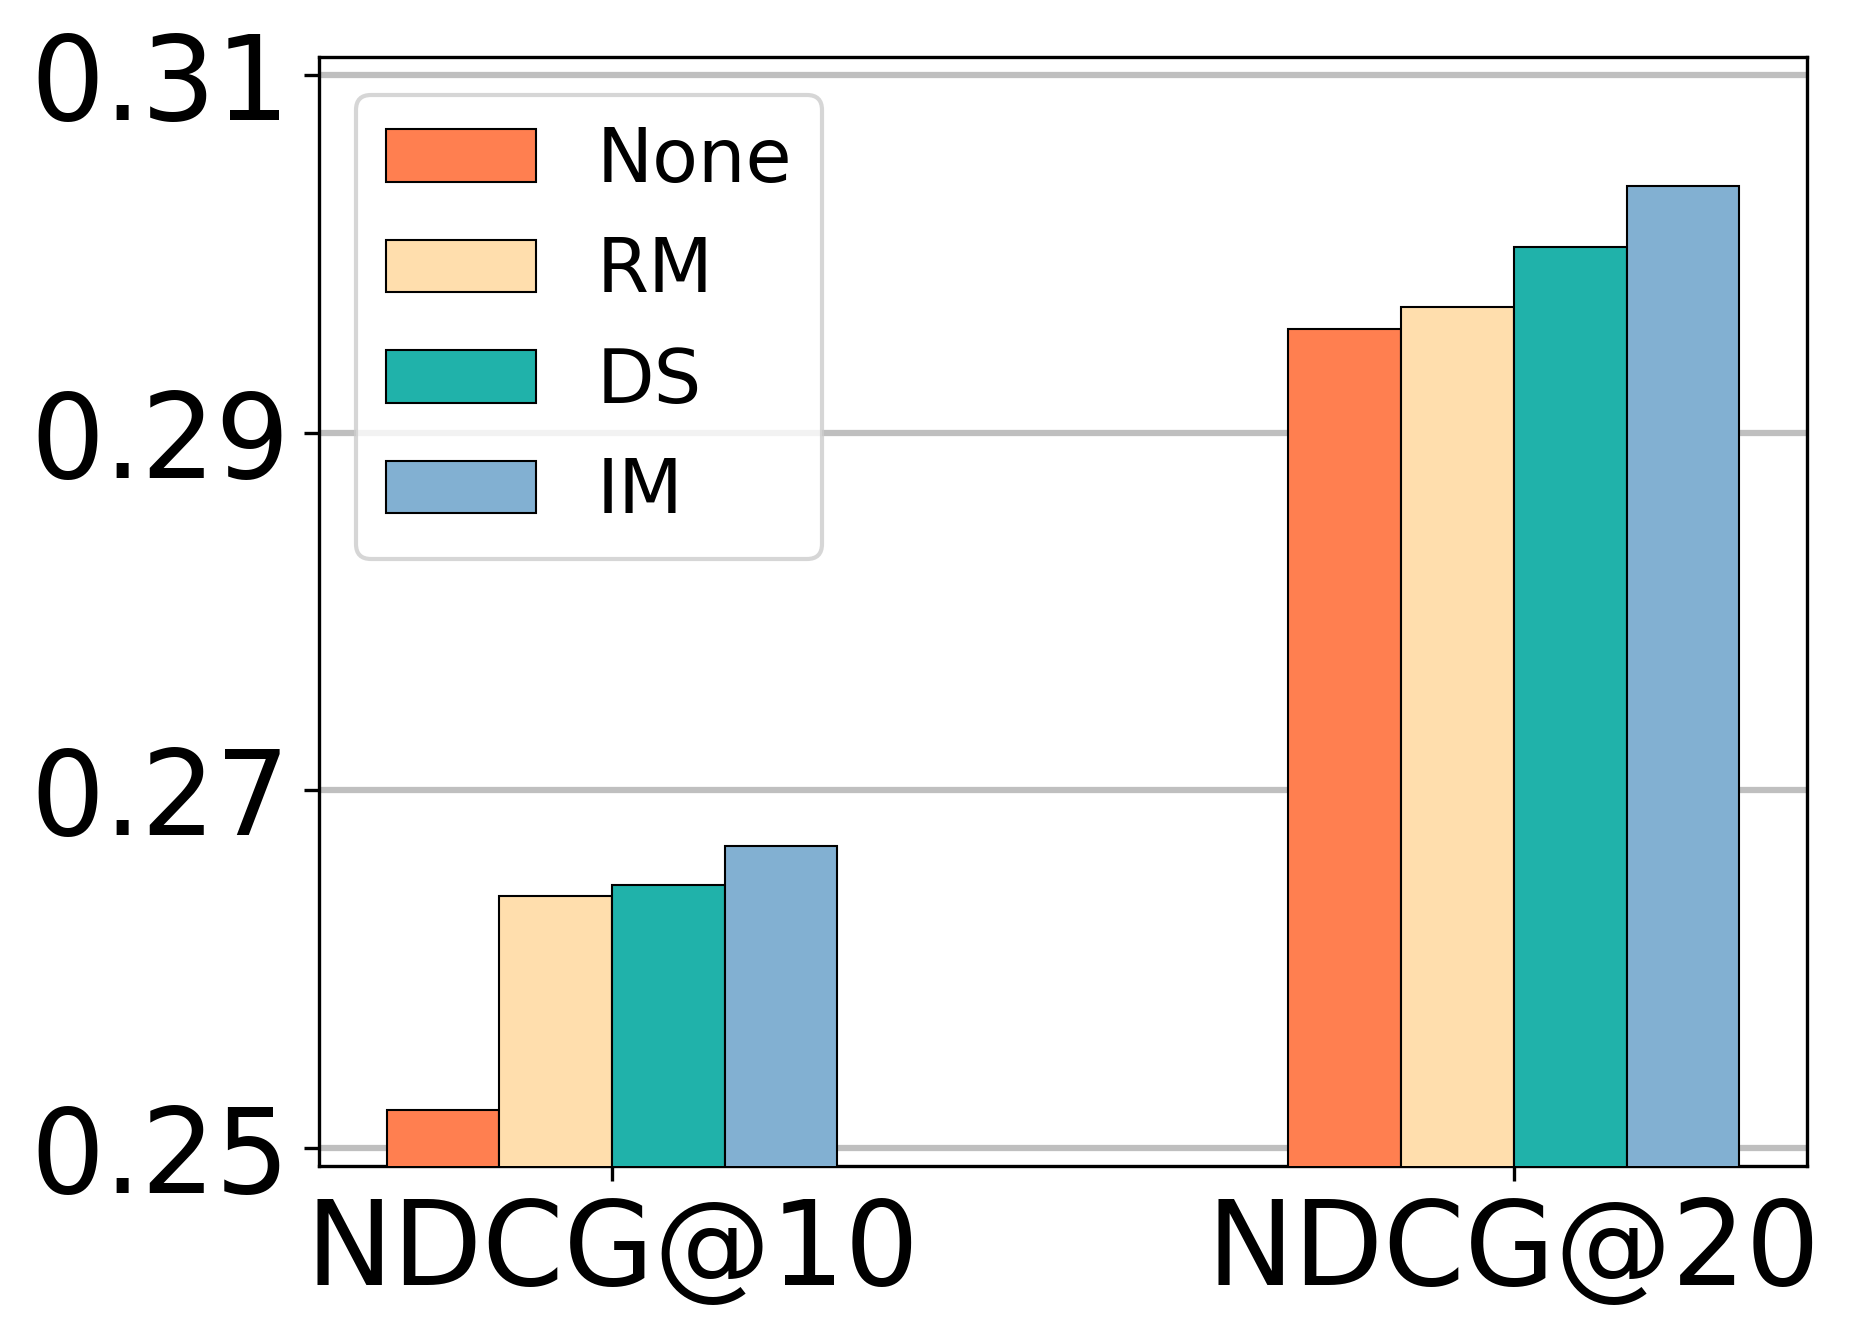}
    \end{minipage}
}
\vspace{-10pt}
\caption{Test on the Mimic Learning.}
\label{mimimi}
\end{wrapfigure}
Next, we test the effectiveness of these three ways (RS: Random Mask, DS: Distribution Shift and IM: Inactive Mixture), and the relative results are given in Fig.~\ref{mimimi}, where $\textit{NDCG@10}$ and $\textit{NDCG@20}$ on Flickr and Yelp are reported. In the figure, `None' means we do not use mimic learning. As shown in figure, all of three designed versions can perform better than `None', which indicates the effectiveness of this component. Among these ways, `Inactive Mixture' constantly outperforms the other two ways, because this way allows the direct mixture of inactive and active embeddings, so that the pseudo inactive users are more similar to the real ones.
